# Supplementary material for: CNC-Net: Self-Supervised Learning for CNC Machining Operations
Source: arXiv:2312.09925 source file (2023-12-15)
Supplement: Supplementary file 6 [file zero_vs_fine_supp.tex]

\begin{figure*}[h]
     \centering
     %%%%%%%%%%%%%%%%%%%%%%%%%%%
     \rotatebox[origin=lB]{90}{\bf Zero-shot}
     \hfill
    \begin{subfigure}[b]{0.12\linewidth}
        \centering
        \includegraphics[trim={0 0 0 0},clip,width=\linewidth, page=1]{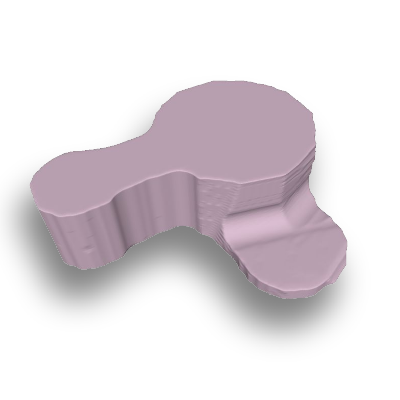}
     \end{subfigure}
     \hfill
     \begin{subfigure}[b]{0.12\linewidth}
        \centering
        \includegraphics[trim={0 0 0 0},clip,width=\linewidth, page=1]{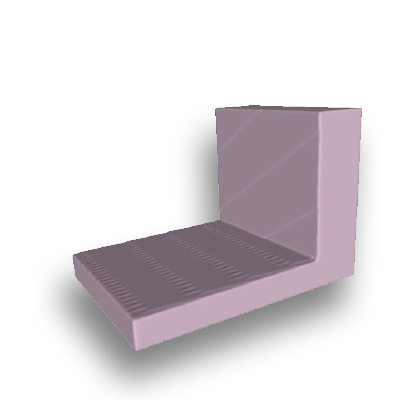}
     \end{subfigure}
     \hfill
     \begin{subfigure}[b]{0.12\linewidth}
        \centering
        \includegraphics[trim={0 0 0 0},clip,width=\linewidth, page=1]{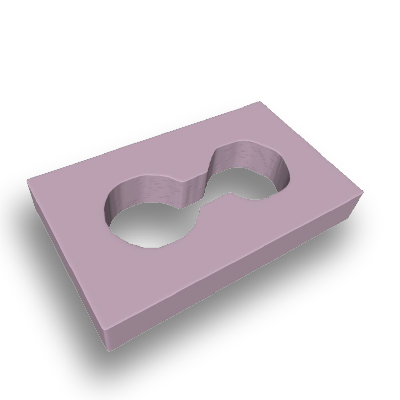}
     \end{subfigure}
     \hfill
     \begin{subfigure}[b]{0.12\linewidth}
        \centering
        \includegraphics[trim={0 0 0 0},clip,width=\linewidth, page=1]{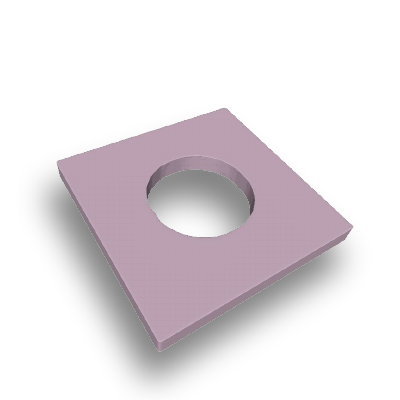}
     \end{subfigure}
     \hfill
     \begin{subfigure}[b]{0.12\linewidth}
        \centering
        \includegraphics[trim={0 0 0 0},clip,width=\linewidth, page=1]{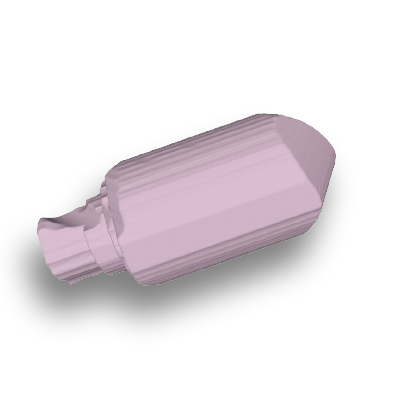}
     \end{subfigure}
     \hfill
     \begin{subfigure}[b]{0.12\linewidth}
        \centering
        \includegraphics[trim={0 0cm 0 0},clip,width=\linewidth, page=1]{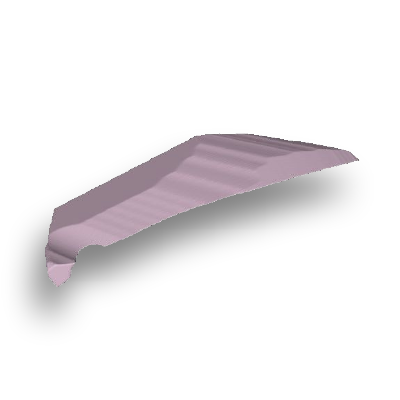}
     \end{subfigure}
     %%%%%%%%%%%%%%%%%%%%%%%%%%
     
     %%%%%%%%%%%%%%%%%%%%%%%%%%
     \rotatebox[origin=lB]{90}{\bf Fine-tuning}
     \hfill
     \begin{subfigure}[b]{0.12\linewidth}
        \centering
        \includegraphics[trim={0 0 0 0},clip,width=\linewidth, page=2]{figures/zero_1.pdf}
     \end{subfigure}
     \hfill
     \begin{subfigure}[b]{0.12\linewidth}
        \centering
        \includegraphics[trim={0 0 0 0},clip,width=\linewidth, page=2]{figures/zero_2.pdf}
     \end{subfigure}
     \hfill
     \begin{subfigure}[b]{0.12\linewidth}
        \centering
        \includegraphics[trim={0 0 0 0},clip,width=\linewidth, page=2]{figures/zero_3.pdf}
     \end{subfigure}
     \hfill
     \begin{subfigure}[b]{0.12\linewidth}
        \centering
        \includegraphics[trim={0 0 0 0},clip,width=\linewidth, page=2]{figures/zero_4.pdf}
     \end{subfigure}
     \hfill
     \begin{subfigure}[b]{0.12\linewidth}
        \centering
        \includegraphics[trim={0 0 0 0},clip,width=\linewidth, page=2]{figures/zero_5.pdf}
     \end{subfigure}
     \hfill
     \begin{subfigure}[b]{0.12\linewidth}
        \centering
        \includegraphics[trim={0 0 0 0},clip,width=\linewidth, page=2]{figures/zero_6.pdf}
     \end{subfigure}
     %%%%%%%%%%%%%%%%%%%%%%%%%%% 

     %%%%%%%%%%%%%%%%%%%%%%%%%%
     \rotatebox[origin=lB]{90}{\bf Target~(GT)}
     \hfill
     \begin{subfigure}[b]{0.12\linewidth}
        \centering
        \includegraphics[trim={0 0 0 0},clip,width=\linewidth, page=3]{figures/zero_1.pdf}
     \end{subfigure}
     \hfill
     \begin{subfigure}[b]{0.12\linewidth}
        \centering
        \includegraphics[trim={0 0 0 0},clip,width=\linewidth, page=3]{figures/zero_2.pdf}
     \end{subfigure}
     \hfill
     \begin{subfigure}[b]{0.12\linewidth}
        \centering
        \includegraphics[trim={0 0 0 0},clip,width=\linewidth, page=3]{figures/zero_3.pdf}
     \end{subfigure}
     \hfill
     \begin{subfigure}[b]{0.12\linewidth}
        \centering
        \includegraphics[trim={0 0 0 0},clip,width=\linewidth, page=3]{figures/zero_4.pdf}
     \end{subfigure}
     \hfill
     \begin{subfigure}[b]{0.12\linewidth}
        \centering
        \includegraphics[trim={0 0 0 0},clip,width=\linewidth, page=3]{figures/zero_5.pdf}
     \end{subfigure}
     \hfill
     \begin{subfigure}[b]{0.12\linewidth}
        \centering
        \includegraphics[trim={0 0 0 0},clip,width=\linewidth, page=3]{figures/zero_6.pdf}
     \end{subfigure}
     %%%%%%%%%%%%%%%%%%%%%%%%%%%  
        \caption{
        \textbf{Qualitative results for zero-shot Vs. fine-tuning} 
        }
        \label{fig:zero_vs_fine_supp}
        \vspace{-4mm}
\end{figure*}
